# Supplementary material for: Securing 5G Bootstrapping: A Two-Layer IBS Authentication Protocol
Source: arXiv:2502.04915 source file (2025-02-07)
Supplement: Supplementary file 1 [file appendix.tex]

\section{Proof of Theorem \ref{thm:eucma}}
\label{thm:proof}

\noindent {\em \small  PROOF.}
 $\mathcal{R}_1$ captures the case where \A~makes at least one signature query during the simulation phase for the target identity and the embedded challenge value is included in the output of \osi. In this reduction algorithm, the ECDLP instance $aP $ is embedded in the commitment value of the signature $R$ instead of the key.   $\mathcal{R}_1$ uses the generalized forking lemma \cite{DBLP:conf/ccs/BellareN06} and the knowledge of the private key of all the users, except the target user  $ID^*$, to obtain a set of two congruences and two unknowns to solve for $a$.  This is done by partitioning the identity space into two disjoint sets $\mathcal{I}_{Ex}$  and $\mathcal{I}_{S}$ randomly. The reduction algorithm can respond to both extract and signature queries for the identities in  $\mathcal{I}_{Ex}$. However, for identities in $\mathcal{I}_{S}$, it aborts on any extract queries, but it can respond to signature queries.  

The reduction algorithm  $\mathcal{R}_2$ uses the multiple forking lemma \cite{DBLP:journals/joc/BoldyrevaPW12} and captures the complement of the above event. More precisely, $\mathcal{R}_2$ captures the case where \A~does not make a signature query on the target user $ID^*$, or  $Q_{ID^*}$ was never returned as a part of the signature query for $ID^*$. Therefore, the ECDLP challenge is embedded in the master public key ($mpk$). For this event, we need to assume that \A~makes a query on $\hash_2$ for $ID^*$, before a $\hash_1$ query is made on $ID^*$. To respond to \osi~queries, \Chall~uses it accesses to the random oracles to simulate the signatures (similar to the simulation of Schnorr signatures) on $ID^*$. However, note that if final forgeries of \A~contain $Q_{ID^*}$ from such sign algorithm, it will not contain the answer to the ECDLP. However, the assumption above   $\mathcal{R}_2$, ensures this does not happen. This reduction uses multiple-forking lemma \cite{DBLP:journals/joc/BoldyrevaPW12} to solve for $a$. 

$\mathcal{R}_3$  algorithm works in the event that \A~does not make a signature query on $ID^*$, or  $Q_{ID^*}$ was never returned as a part of the signature query for $ID^*$ and \A~makes a query on $\hash_1$    for $ID^*$, before a $\hash_2$ query is made on $ID^*$.  The main difference between  $\mathcal{R}_2$ and  $\mathcal{R}_3$ is that in  $\mathcal{R}_3$, the multiple-forking lemma is invoked for four iterations to obtain a set of four congruences and four unknowns to solve for $a$.

Note that the simulation of the reduction algorithms above will be indistinguishable from the real world, by utilizing the random oracles to respond to \A's queries. 

\section{Formal Verification}
\label{Formal Verification}
\noindent We  verify the correctness of our authentication protocol using an automated cryptographic protocol verifier, ProVerif~\cite{proverif}. We consider the Dolev-Yao model~\cite{dolev1983security} (see Section~\ref{Overview}). ProVerif takes as input the description of our proposed protocol specifications in applied $\pi$-calculus dialect~\cite{abadi2001mobile}, and the security and privacy properties, such as secrecy, authenticity and observational equivalences that we want to verify. ProVerif specifications in applied $\pi$-calculus are then translated  into corresponding Horn clauses and property verification is performed through logical derivation by applying resolution techniques used in logic programming. 

\noindent\textbf{Modeling choices.} We model the legitimate participants, such as cellular device, base station, AMF, and the core-PKG in the core network as processes. We use a term algebra to model messages, and equational theory to model algebraic properties of cryptographic primitives. We consider an infinite set of names to represent keys, IDs, and nonces. 

\noindent\textbf{Properties.} We evaluate the following security properties:
\noindent - Secrecy for the private keys of the core-PKG, AMF and base station.

\noindent - Weak authentication (i.e., correspondence) and strong authentication (i.e., injective-correspondence) properties to verify the authenticity and replay protections for the SIB1 message broadcast by base station to the cellular device.

\noindent - Authenticity of the base station's key to the cellular device to ensure that the key is generated by the legitimate AMF.

\noindent - Authenticity of the AMF's key to the cellular device to ensure that the key is generated by the legitimate core-PKG.

\noindent\textbf{Results.} We provide the code for the Proverif formal verification below. ProVerif indeed provided no counter-examples for the above properties and thus signifies the correctness of our proposed authentication protocol.

\subsection{Proverif Code}
\label{proverif_code}

\newcommand{\kwl}[1]{\mathbf{#1}}
\newcommand{\kwf}[1]{\mathsf{#1}}
\newcommand{\kwc}[1]{\mathsf{#1}}

\newcommand{\kwt}[1]{\mathsf{#1}}
\newcommand{\kwe}[1]{\mathsf{#1}}

\newcommand{\var}[1]{\mathit{#1}}

\begin{tabbing}
$\textit{(* Communication channels between PKG, AMF, BS and UE*)} $\\
$\kwl{free}\ \kwc{pkg{\_}to{\_}amf}{:}\ \kwt{channel}\ [\var{private}]. $\\
$\kwl{free}\ \kwc{amf{\_}to{\_}bs}{:}\ \kwt{channel}\ [\var{private}]. $\\
$\kwl{free}\ \kwc{bs{\_}to{\_}ue}{:}\ \kwt{channel}. $\\
$ $\\
$\textit{(*==============================================*)} $\\
$\textit{(*==============================================*)} $\\
$ $\\
$\textit{(*Data Types*)} $\\
$\kwl{type}\ \kwt{nonce}. $\\
$\kwl{type}\ \kwt{public{\_}key}. $\\
$\kwl{type}\ \kwt{secret{\_}key}. $\\
$\kwl{type}\ \kwt{ID}. $\\
$ $\\
$\textit{(*==============================================*)} $\\
$\textit{(*==============================================*)} $\\
$ $\\
$\textit{(*Functions*)} $\\
$ $\\
$\textit{(* Get public key for a particular secret key *)} $\\
$\kwl{fun}\ \kwf{get{\_}public{\_}key}(\kwt{secret{\_}key}){:}\ \kwt{public{\_}key}. $\\
$ $\\
$\textit{(* Generate public key from a nonce *)} $\\
$\kwl{fun}\ \kwf{generate{\_}public{\_}key}(\kwt{nonce}){:}\ \kwt{public{\_}key}. $\\
$ $\\
$\textit{(* Generate secret key based on ID, parent secret key and nonce *)} $\\
$\textit{(* This function is abstracted for simplicity*)} $\\
$\kwl{fun}\ \kwf{generate{\_}secret{\_}key}(\kwt{secret{\_}key}, \kwt{ID}, \kwt{nonce}){:}\ \kwt{secret{\_}key}. $\\
$ $\\
$\textit{(* Sign a message using Schnorr-HIBS scheme *)} $\\
$\kwl{fun}\ \kwf{hibs{\_}sign}(\kwt{bitstring}, \kwt{secret{\_}key}){:}\ \kwt{bitstring}. $\\
$ $\\
$ $\\
$\textit{(*==============================================*)} $\\
$\textit{(*==============================================*)} $\\
$ $\\
$\textit{(* Destructors *)} $\\
$ $\\
$\textit{(* Verify the signature of a message*)} $\\
$\kwl{reduc}\ \kwl{forall}\ \var{m}{:}\ \kwt{bitstring}, \var{k}{:}\ \kwt{secret{\_}key};\  $\\
$\qquad\qquad \kwf{checksign}(\var{hibs{\_}sign}(\var{m}, \var{k}), \kwf{get{\_}public{\_}key}(\var{k})) = \var{m}. $\\
$ $\\
$\textit{(* Verify the public key using parent public key*)} $\\
$\kwl{reduc}\ \kwl{forall}\ \var{k}{:}\ \kwt{secret{\_}key}, \var{xID}{:}\ \kwt{ID}, \var{rand}{:}\ \kwt{nonce};\  $\\
$\qquad\qquad \kwf{parentkey}(\kwf{get{\_}public{\_}key}(\kwf{generate{\_}secret{\_}key}(\var{k},  $\\
$\qquad\qquad \qquad\qquad \qquad\qquad \qquad\qquad \var{xID}, \var{rand}))) = \var{k}. $\\
$ $\\
$ $\\
$\textit{(*==============================================*)} $\\
$\textit{(*==============================================*)} $\\
$ $\\
$\textit{(* Secrecy queries *)} $\\
$ $\\
$\textit{(*Attacker should not have access to the private keys*)} $\\
$\kwl{free}\ \kwc{secret{\_}key{\_}pkg}, \kwc{secret{\_}key{\_}amf},  $\\
$\qquad\qquad \kwc{secret{\_}key{\_}bs}{:}\ \kwt{secret{\_}key}\ [\var{private}]. $\\
$ $\\
$\kwl{query}\ \var{attacker}(\kwc{secret{\_}key{\_}pkg}); $\\
$\ \ \ \ \ \ \var{attacker}(\kwc{secret{\_}key{\_}amf}); $\\
$\ \ \ \ \ \ \var{attacker}(\kwc{secret{\_}key{\_}bs}). $\\
$ $\\
$ $\\
$\textit{(*==============================================*)} $\\
$\textit{(*==============================================*)} $\\
$ $\\
$\textit{(* Authentication queries *)} $\\
$\kwl{event}\ \kwe{authentication{\_}successful}(\kwt{public{\_}key}). $\\
$\kwl{event}\ \kwe{begin{\_}signing}(\kwt{public{\_}key}). $\\
$ $\\
$ $\\
$\kwl{query}\ \var{x}{:}\ \kwt{public{\_}key};\ \kwl{inj\textbf{-}event}(\kwe{authentication{\_}successful}(\var{x}))\  $\\
$\qquad\qquad \Longrightarrow\kwl{inj\textbf{-}event}(\kwe{begin{\_}signing}(\var{x})). $\\
$ $\\
$ $\\
$\textit{(*==============================================*)} $\\
$\textit{(*Core{\_}PKG process*)} $\\
$\kwl{let}\ \var{Core{\_}PKG}(\kwc{secret{\_}key{\_}pkg}{:}\ \kwt{secret{\_}key}) =  $\\
$\qquad\qquad \textit{(*Generate Keys for AMF*)} $\\
$\qquad\qquad \kwl{in}(\kwc{pkg{\_}to{\_}amf}, \var{ID{\_}AMF}{:}\ \kwt{ID}); $\\
$\qquad\qquad \kwl{new}\ \var{rand}{:}\ \kwt{nonce}; $\\
$\qquad\qquad \kwl{let}\ \var{public{\_}key{\_}amf} = \kwf{generate{\_}public{\_}key}(\var{rand})\ \kwl{in} $\\
$\qquad\qquad \qquad\qquad \kwl{out}(\kwc{pkg{\_}to{\_}amf}, (\var{public{\_}key{\_}amf},  $\\
$ \qquad\qquad \qquad\qquad \kwf{generate{\_}secret{\_}key}(\kwc{secret{\_}key{\_}pkg},  $\\
$ \qquad\qquad \qquad\qquad \var{ID{\_}AMF}, \var{rand}))). $\\
$ $\\
$\textit{(*==============================================*)} $\\
$\textit{(*AMF process*)} $\\
$\kwl{let}\ \var{AMF}() =  $\\
$\qquad\qquad \textit{(*Get new keys generated by Core{\_}PKG*)} $\\
$\qquad\qquad \kwl{new}\ \var{ID{\_}AMF}{:}\ \kwt{ID}; $\\
$\qquad\qquad \kwl{out}(\kwc{pkg{\_}to{\_}amf}, \var{ID{\_}AMF}); $\\
$\qquad\qquad \kwl{in}(\kwc{pkg{\_}to{\_}amf}, (\var{public{\_}key{\_}amf}{:}\ \kwt{public{\_}key},  $\\
$\qquad\qquad \qquad\qquad \qquad\qquad \kwc{secret{\_}key{\_}amf}{:}\ \kwt{secret{\_}key})); $\\
$ $\\
$\qquad\qquad \textit{(*Generate keys for the base stations*)} $\\
$\qquad\qquad \kwl{in}(\kwc{amf{\_}to{\_}bs}, \var{ID{\_}BS}{:}\ \kwt{ID}); $\\
$\qquad\qquad \kwl{new}\ \var{rand}{:}\ \kwt{nonce}; $\\
$\qquad\qquad \kwl{let}\ \var{public{\_}key{\_}bs} = \kwf{generate{\_}public{\_}key}(\var{rand})\ \kwl{in} $\\
$\qquad \qquad\qquad \kwl{out}(\kwc{amf{\_}to{\_}bs}, (\var{public{\_}key{\_}bs},  $\\
$\qquad \qquad\qquad \kwf{generate{\_}secret{\_}key}(\kwc{secret{\_}key{\_}amf}, \var{ID{\_}BS}, \var{rand}),  $\\
$\qquad\qquad \qquad\qquad \var{ID{\_}AMF}, \var{public{\_}key{\_}amf}\ )). $\\
$ $\\
$\textit{(*==============================================*)} $\\
$ $\\
$\textit{(*base station process*)} $\\
$\kwl{let}\ \var{BS}() =  $\\
$\qquad\qquad \textit{(*Get new keys generated by AMF*)} $\\
$\qquad\qquad \kwl{new}\ \var{ID{\_}BS}{:}\ \kwt{ID}; $\\
$\qquad\qquad \kwl{out}(\kwc{amf{\_}to{\_}bs}, \var{ID{\_}BS}); $\\
$\qquad\qquad \kwl{in}(\kwc{amf{\_}to{\_}bs}, (\var{public{\_}key{\_}bs}{:}\ \kwt{public{\_}key},  $\\
$\qquad\qquad \qquad\qquad \kwc{secret{\_}key{\_}bs}{:}\ \kwt{secret{\_}key}, \var{ID{\_}AMF}{:}\ \kwt{ID},  $\\
$\qquad\qquad \qquad\qquad \var{public{\_}key{\_}amf}{:}\ \kwt{public{\_}key})); $\\
$ $\\
$\qquad\qquad \textit{(*Sign the SIB1 message*)} $\\
$\qquad\qquad \kwl{new}\ \var{SIB1}{:}\ \kwt{bitstring}; $\\
$\qquad\qquad \kwl{event}\ \kwe{begin{\_}signing}(\var{public{\_}key{\_}bs}); $\\
$\qquad\qquad \kwl{let}\ \var{sig{\_}SIB1} = \var{hibs{\_}sign}(\var{SIB1}, \kwc{secret{\_}key{\_}bs})\ \ \kwl{in} $\\
$\qquad\qquad \qquad\qquad \kwl{out}(\kwc{bs{\_}to{\_}ue}, (\var{SIB1}, \var{sig{\_}SIB1}, \var{ID{\_}BS}, \var{ID{\_}AMF},  $\\
$\qquad\qquad \qquad\qquad \qquad\qquad \var{public{\_}key{\_}bs}, \var{public{\_}key{\_}amf})). $\\
$ $\\
$\textit{(*==============================================*)} $\\
$ $\\
$\textit{(*UE process*)} $\\
$\kwl{let}\ \var{UE}(\var{public{\_}key{\_}pkg}{:}\ \kwt{public{\_}key}) =  $\\
$\qquad\qquad \textit{(*Receive and verify signature*)} $\\
$\qquad\qquad \kwl{in}(\kwc{bs{\_}to{\_}ue}, (\var{SIB1}{:}\ \kwt{bitstring}, \var{sig{\_}SIB1}{:}\kwt{bitstring},  $\\
$\qquad \qquad\qquad \var{ID{\_}BS}{:}\ \kwt{ID}, \var{ID{\_}AMF}{:}\ \kwt{ID}, \var{public{\_}key{\_}bs}{:}\ \kwt{public{\_}key},  $\\
$\qquad \qquad\qquad \var{public{\_}key{\_}amf}{:}\ \kwt{public{\_}key})); $\\
$ $\\
$\qquad\qquad \textit{(* Check whether signature is valid*)} $\\
$\qquad\qquad \kwl{let}\ ( = \var{SIB1}) = \kwf{checksign}(\var{sig{\_}SIB1}, \var{public{\_}key{\_}bs})\ \kwl{in} $\\
$\qquad\qquad \textit{(* Verify BS's public key*)} $\\
$\qquad\qquad \kwl{let}( = \var{public{\_}key{\_}amf}) = \kwf{get{\_}public{\_}key}( $\\
$\qquad\qquad \qquad\qquad \qquad\qquad  \kwf{parentkey}(\var{public{\_}key{\_}bs}))\ \kwl{in} $\\
$\qquad\qquad \textit{(* Verify AMF's public key*)} $\\
$\qquad\qquad \kwl{let}( = \var{public{\_}key{\_}pkg}) = \kwf{get{\_}public{\_}key}( $\\
$\qquad\qquad \qquad\qquad  \kwf{parentkey}(\var{public{\_}key{\_}amf}))\ \kwl{in} $\\
$\qquad\qquad \kwl{event}\ \kwe{authentication{\_}successful}(\var{public{\_}key{\_}bs}). $\\
$ $\\
$\textit{(*==============================================*)} $\\
$\textit{(*==============================================*)} $\\
$\textit{(* Main process*)} $\\
$\kwl{process} $\\
$\qquad\qquad \textit{(* Generate PKG's secret key*)} $\\
$\qquad\qquad \kwl{new}\ \kwc{secret{\_}key{\_}pkg}{:}\ \kwt{secret{\_}key}; $\\
$\qquad\qquad  $\\
$\qquad\qquad \textit{(* Start all individual processes in parallel*)} $\\
$\qquad\qquad (\var{Core{\_}PKG}(\kwc{secret{\_}key{\_}pkg})\mid $\\
$\qquad\qquad \qquad\qquad \qquad \ !\var{AMF}()\mid $\\
$\qquad\qquad \qquad\qquad \qquad !\var{BS}()\mid $\\
$\qquad\qquad \qquad\qquad \qquad !\var{UE}(\kwf{get{\_}public{\_}key}(\kwc{secret{\_}key{\_}pkg}))) $\\

\end{tabbing}

\section{Evaluation on a cellular device}

\begin{table}[!h]
\begin{tabular}{|c||c|c|c|c|}
\hline
\multirow{2}{*}{\textbf{Scheme}} & \multicolumn{2}{c|}{\textbf{Sign}}   & \multicolumn{2}{c|}{\textbf{Verify}} \\ \cline{2-5} 
 & \multicolumn{1}{l|}{ms} & \multicolumn{1}{l|}{Cycles} & \multicolumn{1}{l|}{ms} & \multicolumn{1}{l|}{Cycles} \\ \hline
BLS~\cite{boneh2001short} & 1.24 & 2.48 & 12.98 & 25.97 \\ \hline
ECDSA-256~\cite{johnson2001elliptic} & 0.94 & 1.88 & 2.94 & 5.89 \\ \hline
SCRA-BGLS~\cite{yavuz2017real} & 0.11 & 0.23 & 17.14 & 342.81 \\ \hline
BLMQ~\cite{IEEE1363} & 1.24 & 2.48 & 14.53 & 29.07 \\ \hline
SM9~\cite{cheng2017sm9} & 1.86 & 3.72 & 8.55 & 17.10 \\ \hline \hline
Schnorr-HIBS & 0.02 & 0.05 & 1 & 2.00 \\ \hline
Schnorr-HIBS-P & 0.01 & 0.02 & 1 & 2.00 \\ \hline
\end{tabular}

\begin{tablenotes}[flushleft] 
 \footnotesize{
We estimate the signing and verification performance of all the schemes by assuming a cellular device with a CPU clock speed of 2 GHz. All computations are in milliseconds and CPU cycles are in millions.}
\end{tablenotes}
\caption{Comparison of the signing and verification of the candidate signature schemes for authenticating cellular base stations on cellular device.}	
\label{eval_cellular}
\end{table}
